# Supplementary material for: Long-Baseline Neutrino Facility (LBNF) and Deep Underground Neutrino Experiment (DUNE) Conceptual Design Report Volume 2: The Physics Program for DUNE at LBNF
Source: arXiv:1512.06148 source file (2016-01-22)
Supplement: Supplementary file 1 [file supp-doc-list.tex]

%\chapter{Supporting Documents}
% AH 12/30/11: Since I'm pulling this in as a chapter in vol 1 and as a subsection in section 1.1 of vols 2-6, I'm taking the chapter heading out and putting it directly into the file that inputs all the content of volume 1
A host of information related to the CDR is available in a set of supporting documents. Detailed information on risk analysis and mitigation, value engineering, ES\&H, costing, project management and other topics not directly in the design scope can be found in these documents, listed in 
Table~\ref{table:cd-1-doc-list}. Each document is numbered and stored in LBNE's document database, accessible via a username/password combination provided by the Project. Project documents stored in this database are made available to internal and external review committees through Web sites developed to support individual reviews.

%\fixme{Either need descriptions, or get rid of Description column; need to finalize table. AH}

\begin{center}
\begin{longtable}{|p{10cm}|p{4cm}|} %{|l|l|l|}
\caption{LBNE CD-1 Documents}
\label{table:cd-1-doc-list} \\
   \multicolumn{1}{p{10cm}}{\textbf{Title}} & % 2/23/12 AH tried upping col width from 5 and 2.
   \multicolumn{1}{p{4cm}}{\textbf{LBNE Doc Number(s)}} \\
\hline
\endfirsthead
Acquisition Plan & 5329 \\
\hline
Alternatives Analysis  & 4382    \\
\hline
Case Study Report; Liquid Argon TPC Detector &  3600   \\
\hline
Configuration Management Plan & 5452  \\
\hline
DOE Acquisition Strategy for LBNE & 5442 \\
\hline
Integrated Environment, Safety and Health Management Plan & 4514 \\
\hline
LAr-FD Preliminary ODH Analysis &  2478   \\
\hline
Global Science Objectives, Science Requirements and Traceback Reports &  4772   \\
\hline
Preliminary Hazard Analysis Report  &  4513  \\
\hline
Preliminary Project Execution Plan &   5443 \\
\hline
Preliminary Security Vulnerability Assessment Report & 4826 \\
\hline
Project Management Plan  & 2453    \\
\hline
Project Organization Chart & 5449    \\
\hline
Quality Assurance Plan & 2449    \\
\hline
Report on the Depth Requirements for a Massive Detector at Homestake & 0034  \\
\hline
Requirements, Beamline &  4835   \\
\hline
Requirements (Parameter Tables), Far Detector &  3747 (3383)\\
\hline
Requirements, Far Site Conventional Facilities  &   4408  \\
\hline
Requirements, Near Detectors & 5579 \\
\hline
Requirements, Near Site Conventional Facilities & 5437  \\
\hline
Risk Management Plan & 5749    \\
\hline
Value Engineering Report & 3082   \\
\hline
Work Breakdown Structure (WBS) & 4219    \\
\hline
%Cost Book List, Beamline &  http://lbne.fnal.gov/reviews/beam-costbooklist.shtml  \\
%\hline
%Cost Book List, Near Detector & http://lbne.fnal.gov/reviews/nd-costbooklist.shtml  \\
%\hline
%Cost and Schedule documents, LAr-FD &  5131  \\
%\hline
%\end{tabular} 
\end{longtable}
\end{center}
